# Supplementary material for: Stability of space-time isogeometric methods for wave propagation problems
Source: arXiv:2303.15460 source file (2023-03-11)
Supplement: Supplementary file 3 [file AppendixTemplate.tex]

% Appendix Template

\chapter{Appendix Title Here} % Main appendix title

\label{AppendixX} % Change X to a consecutive letter; for referencing this appendix elsewhere, use \ref{AppendixX}

Write your Appendix content here.
